# Supplementary material for: Divide-and-Conquer for Lane-Aware Diverse Trajectory Prediction
Source: arXiv:2104.08277 source file (2021-04-16)
Supplement: Supplementary file 1 [file supp_dac_non_uniform.tex]

\begin{figure}[ht]
    \centering
    \begin{subfigure}{0.24\linewidth}
        \includegraphics[width=\linewidth]{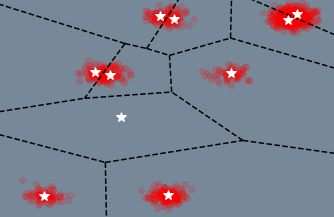}
        \caption{EWTA}
        % \label{fig:toy_dac_init}
    \end{subfigure}
    \begin{subfigure}{0.24\linewidth}
        \includegraphics[width=\linewidth]{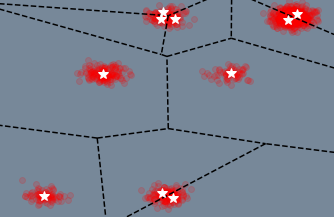}
        \caption{DAC}
        % \label{fig:toy_dac_wta}
    \end{subfigure}
    \begin{subfigure}{0.24\linewidth}
        \includegraphics[width=\linewidth]{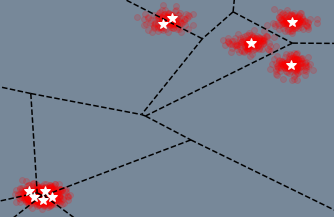}
        \caption{EWTA}
        % \label{fig:toy_dac_rwta}
    \end{subfigure}
    \begin{subfigure}{0.24\linewidth}
        \includegraphics[width=\linewidth]{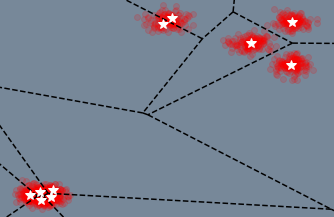}
        \caption{DAC}
        % \label{fig:toy_dac_ewta}
    \end{subfigure}
   
    \caption{
    }
    \label{fig:dac_non_uniform}
\end{figure}
